# Supplementary material for: On-edge Multi-task Transfer Learning: Model and Practice with Data-driven Task Allocation
Source: arXiv:2107.02466 source file (2021-07-06)
Supplement: Supplementary file 1 [file Appendix.tex]

\appendix
\subsection{Potential Benefit of Allocation based on Importance}

In major industrial AIOps systems, the general industrial process likely to complete a task with low merits for decision making in AIOps at first and try to iteratively improve the decision performance by aggregating the output of a sequence of tasks, where usually consists of two steps, i.e., Data-driven Multi-task Transfer Learning and Final Optimization, and they work as follows. When an industrial demand arrives, AIOps systems first need to choose a series of data-driven prediction tasks to conduct (Data-driven Multi-task Transfer Learning). Then, the AIOps systems receive all the results of previous prediction tasks and conduct decisions until the decision performance, i.e., overall system merit, is no longer improved (Final Optimization). 

To ensure the reliable decision performance, it will consume considerable time and even exceeding the time constraints to blindly conduct all tasks on the edge. However, by using our method that tend to allocate more resources to more important tasks  (shown in Sec. \ref{Sec:Model}), not only industrial performance can be guaranteed but also saves significant resources and time. 

To demonstrate the benefit, we conduct experiments on a real-world \emph{chiller operation} dataset released in \cite{zheng2018data}, which contains four-year operation data for three high-rise office towers in a metropolitan, collected by a major building manage service provider. Chiller is a machine generate cooling power in buildings. The chiller operation aims to select run-time configurations of the chiller so that the overall system serves the cooling demand while minimizes the energy consumption.  

It is worth noting that in our experiment, reliable chiller operation decision depends on the prediction result of each {\em learning task} across all the operations for different chillers, where {\em learning task} refers to cooling-performance prediction of a chiller for one particular operation. At the same time, the chiller operation decision process, like the general industrial process as described above, not only is usually an iterative optimization process but also often accompanied by time limits (e.g., two hours for chiller operations \cite{sun13}). Blindly conducting all the learning tasks leads to consuming considerable time and even exceeding the time limits. Furthermore, tasks that exceed the time limits will not obtain the prediction results, which result in a significant impact on the final decision performance. Note that in the industrial field, when the final decision cannot meet the requirement of the industry, which will lead to a series of additional operations, thus consumes considerable extra energy. \footnote{Annual cost $C$ is calculated as follows: $C = \sum_i E_i \times c_i$, where $E_i$ refers to the electricity consumption after the decision making on day $i$ and $c_i$ denotes the price of electricity on day $i$.}  However, our approach tends to allocate more resources to important learning tasks to make sure they all finish within the time limits, not only industrial performance can be guaranteed but also saves significant resources and time. Finally, our approach saves 35.68\% of the annual electricity cost, i.e., nearly 1.3 million dollar.

\subsection{Supplementary Design of SVM Predictor}

Our idea is to leverage runtime data to adjust the decision of the general predictor with RL. To this end, we propose a local predictor with SVM which serves as an adjuster that leverages all the real-world data. The design of loss function and feature engineering are introduced as follows.

\textbf{1. Loss Function.} Formally, let $\mathcal{R}$ be the training dataset of the real-world data, sample $k \in \mathcal{R}$ usually consists of two parts. One is a vector $x_k$ that is regarded as the input feature values; the other is a scalar $y_k$ that is the desired output of the model. Then, we define the loss function $\mathcal{L}_k(w)$ of our SVM predictor $\mathcal{F}_2(\cdot)$ as follows:
\begin{eqnarray}
\mathcal{L}_k(w) =  \frac{1}{2}\Vert w \Vert ^2 + \frac{1}{2} \textrm{max} \{0; 1 - y_k w^T x_k \} ^2,
\end{eqnarray}
where $w$ denotes its parameter vector; $w^T$ denotes the transpose of $w$ and $\Vert \cdot \Vert ^2$ denotes the $\mathcal{L}^2$ norm.

Finally, our optimization process is to find the optimal parameter vector $w^*$ that minimize the loss function $\mathcal{L}_k(w)$ on a collection of training dataset $\mathcal{R}$. Hence, $w^* = \arg \min \frac{1}{\vert \mathcal{R} \vert}\sum_{k \in \mathcal{R}} \mathcal{L}_k(w)$.

\textbf{2. Feature Engineering.} In most real-world scenarios, e.g., industry domain, it is either costly or even impossible to obtain the data on environments and configurations of tasks; we usually do not have the luxury to obtain enormous data where local predictor can be trained with irrelevant features automatically eliminated. As such the challenge is to select the proper feature set for our local predictor. Thus, we propose a domain-assisted feature engineering approach which uses domain knowledge to create features relevant to the problem at hand. The feature set consists of the following two types of features, naming domain features and general features, respectively.

\begin{itemize}
    \item \textbf{Domain features.} Obviously, the domain features are closely related to the specific scenarios. For example, in driver-less car, driving operation decision is critical to driver-less car safety, which consist of the following specific characteristics such as engine status, speed, radar data, GPS data and etc. While in industrial field, chiller sequencing is a common but highly important industrial operation in energy-efficient buildings, which consists of the following specific characteristics such as operating power, water temperature difference, flow rate, recent cooling load and etc.
    
    \item \textbf{General features.} Overall, the general features should have some universality and can be easily applied to other scenarios. More specifically, it should reflect the decision performance of a data-driven task in the statistical view over the historical data, such as past success, prediction accuracy and etc.
\end{itemize}
